# Supplementary material for: An elasto-plastic approach based on microscopic insights for the steady state and transient dynamics of sheared disordered solids
Source: arXiv:2007.07162 source file (2021-01-08)
Supplement: Supplementary file 1 [file SI_revised.pdf]

# Supplementary Information: An elasto-plastic approach based on microscopic insights for the steady state and transient dynamics of sheared disordered solids

Chen Liu
*Laboratoire de Physique de l'Ecole Normale Supérieure, Paris, France*

Suman Dutta and Pinaki Chaudhuri
*The Institute of Mathematical Sciences, Taramani, Chennai 600113, India*

Kirsten Martens
*Univ. Grenoble Alpes, CNRS, LIPhy, 38000 Grenoble, France*

### Determination of the parameters

In the following, we describe in detail the different parameters involved in the mesoscopic model, their physical interpretation and the procedure to determine these parameters from the microscopic simulations. The typical Maxwell relaxation time for the localised shear transformations has been already estimated $\tau \approx 1$[1]. Other parameters are tuned to achieve consistency between mesoscopic and microscopic simulation results. The parameters we need to determine are:

- Time scales: The typical delay $\tau^{pl}$ of plastic activation once a site overcomes the local threshold $\sigma_i^{th}$, and the typical duration of a local plastic event $\tau^{res}$.
- The typical value of dynamically renewed local threshold $\sigma_d^{th}$, and the exponent $k_d$ that shapes the distribution of the dynamically renewed local threshold.

By tuning these parameters, we try to match the mesoscopic results with the MD simulation results for several types of observables, as discussed in the main text, viz. the flow curve, the load curves at different shear rate, the creep curves at different stresses and the also the steady state threshold distribution $P_a(\sigma^{th})$. As the free parameters form a high dimensional space and the effects of the parameters on observables are highly non-linear, and for each parameter setting we should run a whole set of simulations to compare with the particle based simulation results, it is a heavy and non-trivial task to find the set of correct parameters. However we can make qualitative arguments to understand better the effects of the parameters on observables and then find the appropriate directions for tuning the parameters.

One realizes easily that once the flow curve is well fitted, a good comparison is ensured for the steady state observables, namely the stress plateau of the load curves and the shear rate plateau of the creep curves. Then one can adjust the parameters to match the transient state of the mesoscopic model to the microscopic simulations for both load curves and creep curves, while minimizing the effects on the flow curve. Finally one should take care of the steady state distribution $P_a(\sigma^{th})$. For the last comparison, it is very difficult to get a quantitative match, because the simulation results can only present approximations due to the frozen matrix approach and thus we are satisfied by a qualitative agreement as discussed in the main text. We apply this strategy for parameter tuning with the following arguments describing qualitatively the effects of the parameters on the different types of observables.

Except for the flow curve, where we can have some quantitative indications for the effect of the parameters, we otherwise only have qualitative hints for fitting other the other observables. This is of coarse due to the non-linear nature of the model, which is necessary to reproduce the non-trivial dynamics of a particle based model. By finding a setting of parameters for the mesoscopic model that simultaneously captures the results of the microscopic simulations in all observables, we confirm that the essence of the rheological properties of amorphous systems are indeed encoded in the simple rules of the lattice models, able to encompass the complex macroscopic phenomena for driven disordered materials.

#### *The flow curve*

In this section, we explain our understanding of how the different parameters in the mesoscopic model influences the fitting parameters in the flow curve. For this, we consider for simplicity a typical site sheared at a rate $\dot{\gamma}$. Neglecting the random kicks from plastic events elsewhere, the site alternates between the elastic and the plastic state, with its stress going up and down between two typical values $\sigma_H > \sigma_L$ which are typical stress values for which the state alters. By construction, plastic events can only take place when the stress is above the threshold, the typical value of which is $\sigma_d^{th}$. During the plastic state, the stress drops as

$$\sigma = \mu\tau\dot{\gamma} + (\sigma_H - \mu\tau\dot{\gamma})\exp(-t/\tau)\ . \qquad (1)$$

As the typical duration is $\tau^{res}$, the typical stress at which the site becomes elastic again, is then

$$\sigma_L = \mu\tau\dot{\gamma} + (\sigma_H - \mu\tau\dot{\gamma})\exp(-\tau^{res}/\tau) \qquad (2)$$

Two rheological regimes can be recognized depending on the shear rate $\dot{\gamma}$.

- High shear rate regime. The typical value of $\sigma_L$ is above the typical threshold $\sigma_d^{th}$ due to the high shear rate, so that we have

$$\sigma_L > \sigma_d^{th} \qquad (3)$$
$$\sigma_H = \sigma_L + \mu\tau^{pl}\dot{\gamma} \qquad (4)$$

- Low shear rate regime. The typical value of $\sigma_L$ lies below $\sigma_d^{th}$ during a plastic event, which implies

$$\sigma_L < \sigma_d^{th} \qquad (5)$$
$$\sigma_H = \sigma_d^{th} + \mu\tau^{pl}\dot{\gamma} \qquad (6)$$

After simple computations, we find that the two rheological regimes are separated by a crossover shear rate

$$\dot{\gamma}_X \approx \frac{\sigma_d^{\text{th}}}{\tau\mu}\frac{1-\exp(-\frac{\tau^{res}}{\tau})}{1+(\frac{\tau^{pl}}{\tau}-1)\exp(-\frac{\tau^{res}}{\tau})} \qquad (7)$$

Below this shear rate, the flow curve is complex due to the disorder penalized non-linear local dynamics and this part of the flow curve can be eventually fitted by the Herschel-Buckley law, while above this shear rate, the flow curve becomes linear. Thus $\dot{\gamma}_X$ is the quantity that characterizes the shape of the flow curve.

In the low shear rate regime, we can estimate the dynamical yield stress $\Sigma^Y$, by taking the limit of zero shear rate. In this limit, the rising stress part takes infinite time, while the decrease happens during the duration $\tau^{res}$, so that $\Sigma^Y$ can be estimated as the algebraic average :

$$\Sigma^Y \approx \frac{1}{2}(\sigma_H(\dot{\gamma}=0) + \sigma_L(\dot{\gamma}=0)+) \qquad (8)$$
$$\approx \frac{\sigma_d^{\text{th}}}{2}\left(1+\exp(-\frac{\tau^{res}}{\tau})\right) \qquad (9)$$

This estimation represents the global offset of the flow curve.

During the procedure for fitting the flow curve, the global offset of the flow curve and the scope of power low regime are adjusted by $\Sigma^Y$ and $\dot{\gamma}_X$, with a clarified dependence on the parameters.

*Transient dynamics in the stress-strain curve*

Here we address the parts of the stress-strain curve before entering the steadily flowing state which contains (i) the slope of elasticity for $\gamma \geq 0$, (ii) the rate dependent overshoot height and (iii) the time needed to reach the steady state after the overshoot. The slope is given by $\mu$ which is measured directly from the particle based dynamics, thus giving a good match (main text figures).

The height of the overshoot in the stress-strain curve is reached when a significant portion of sites overcomes their initial thresholds, which is an input from the MD simulations with a typical value, noted as $\sigma_I^{th}$. Given a shear rate $\dot{\gamma}$ the typical stress for a site to yield is then given by

$$\Sigma^{\text{overshoot}} \approx \sigma_I^{th} + \mu\tau^{pl}\dot{\gamma} \qquad (10)$$

Thus the $\tau^{pl}$ is rather uniquely fixed by matching systematically the height of all load curves for different shear rate.

The relaxation to the steady state after the overshoot is related with $\tau^{res}$. Increasing $\tau^{res}$ would give more time to release the stress, shortening the overall duration of the transient regime.

*The transient state of the creep curves*

The fluidization time $\tau_f$ is closely related with the parameter $\tau^{res}$. Increasing $\tau^{res}$ gives sites more time to release their local stresses so that more sites may be activated. Thus overall, the system will fluidize faster for a larger value of $\tau^{res}$.

*The effect of shear modulus*

From the above discussions, we conclude that the shear modulus essentially plays no role in determining the low shear rate power law regime of the flow curve (Eq.8). It only affects the crossover shear rate $\dot{\gamma}_X$ that determines the range of validity of our elasto-plastic model (Eq.7). Increasing the shear modulus only shrinks the range of non trivial power law regime of the flow curve. Fig.1 compares two flow curves produced by the mesoscopic model with two extreme values of the shear modulus used in our work and one flow curve produced by our MD simulation, confirming well the above statement.

The shear modulus, however, does affect the transient behavior such as the slope of stress-strain curves at small deformations and the height of the stress overshoot (Eq.10). In reality, the shear modulus is dependent on the preparation of the initial state and independent in the stationary flowing state, which implies a hidden dynamics of the shear modulus upon external loading that brings the shear modulus from its initial value $\mu(t=0)$ to the steady state value $\mu(t=\infty)$. However the study of the dynamics of the shear modulus due to external

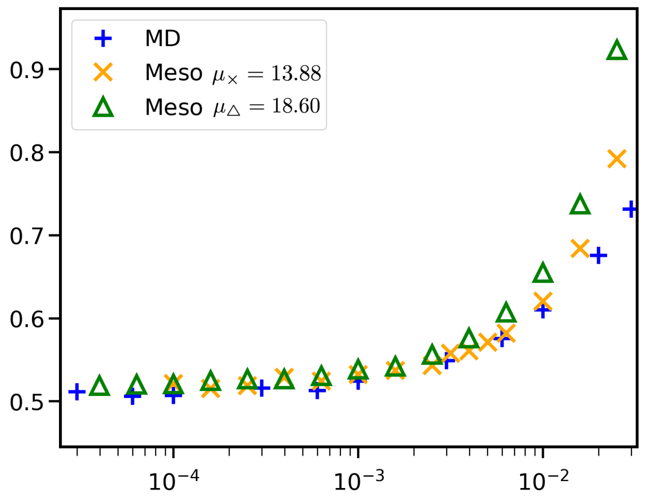


FIG. 1. Check on dependence of flow curves on choice of shear modulus. The MD flow curve is obtained by shearing a $E_1$ sample (see main text for description). The mesoscopic data is obtained by using two different values of shear modulus $\mu_\times \approx 13.88$ and $\mu_\triangle \approx 18.6$. Both meso flow curves agree well with the MD result at low shear rate regime. In the large shear-rate regime, there are deviations from the MD data, with the curve for the higher shear modulus deviating from the MD data at a smaller value than that for the lower shear modulus.

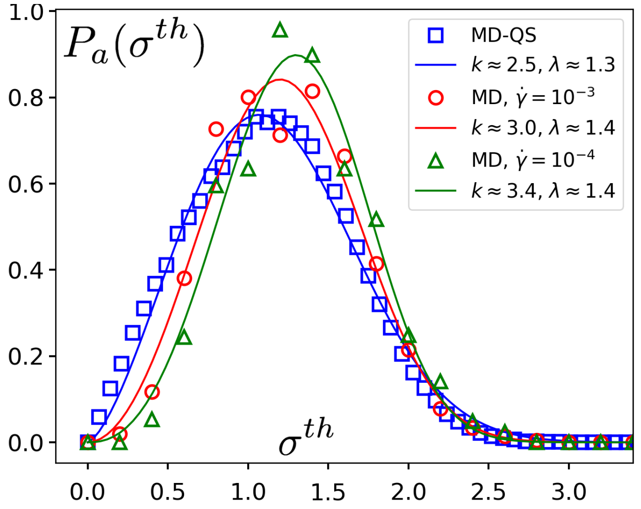


FIG. 2. Open symbols are empirical stationary local threshold distribution $P_a(\sigma^{th})$ measured from MD simulations, where quasi-static data (MD-QS) is obtained from [2] and finite shear rate data is recapped from our main text. Solid lines are corresponding fitted Weibull distributions, where the fitting parameters are indicated in the legend.

driving is scarce in the literature. The property of our mesoscopic model, that the shear modulus affects only the transient behavior without changing the stationary flow curve within the validity domain, allows us to use only the shear modulus of the initial state without introducing extra uncontrolled dynamics, while at the same time, captures both transient and stationary behaviors of our microscopic simulations.

### *The local threshold distribution*

The stationary state local threshold distribution $P_a(\sigma^{th})$ has been measured previously with finite rate simulations [1] and in the quasi-static driving limit [2]. In both cases, as well as for our simulation data, the empirical distributions can be reasonably fitted with a Weibull distribution (see Fig.2)

$$W(x) = \frac{k}{\lambda}\left(\frac{x}{\lambda}\right)^{k-1} \exp\left(-\left(\frac{x}{\lambda}\right)^{k}\right) \qquad (11)$$

.

Since it is difficult to assess directly from MD systems the dynamic threshold distribution $P_d(\sigma^{th})$ which is an important ingredient of the mesoscopic model, we adopt the form of Weibull distribution as an ansatz for $P_d(\sigma^{th})$ (Eq.4 in the main text) to eliminate as much as possible uncontrolled parameters. Besides, as the external loading statistically hardens mescoscopic sites to larger values of $\sigma^{th}$ than the dynamically renewed ones[3], we expect a smaller typical value of the dynamically renewed local threshold than the one in stationary state, i.e. $\sigma_d^{th} < \lambda$, where measured values of $\lambda$, together with $k$, are indicated in Fig.2. With this constraint in mind, we tune the values of $k_d$ and $\sigma_d^{th}$ of Eq.4 in the main text in order to achieve the best overall consistency between meso and MD results.

### Details of molecular dynamics simulations

We consider a two-dimensional binary Lennard Jones mixture of *small* and *large* interacting particles of equal masses which has been demonstrated to be a good glass former and whose mechanical properties have been well studied [2, 4, 5]. The system is studied at a density of 1.02, using $N = 102400$ particles in a two dimensional box of length $L = 316.174$. The ratio of the large (L) and small (S) is given by $\frac{N_L}{N_S} = \frac{1+\sqrt{5}}{4}$ where $N_L$ and $N_S$ are the number of L and S particles respectively. The interaction between any pair of particles having co-ordinates $\mathbf{r}_i$ and $\mathbf{r}_j$, is given by

$$V_{\alpha\beta}(r) = 4\epsilon_{\alpha\beta}\left[(\sigma_{\alpha\beta}/r)^{12} - (\sigma_{\alpha\beta}/r)^{6}\right] . \qquad (12)$$

where $r = |\mathbf{r}_i - \mathbf{r}_j|$, and $\alpha, \beta$ correspond to the identities $S$ or $L$. The values of the interaction parameters are set to $\epsilon_{\rm SL} = 1.0$, $\epsilon_{\rm SS} = \epsilon_{\rm LL} = 0.5\epsilon_{\rm LS}$, $\sigma_{\rm LS} = 1$, $\sigma_{\rm LL} = 2\sin\pi/5$, $\sigma_{\rm ss} == 2\sin\pi/10$. In the following, we use $\epsilon_{\rm LS}$ and $\sigma_{\rm LS}$ as the unit for energy and length, respectively. The cutoff

radius in Eq. (12) is chosen as $R_c = 2.5\sigma_{\rm LS}$ and the potential is smoothened out near the cutoff [2]. As the time unit, we use $\sqrt{m\sigma_{\rm LS}^2/\epsilon_{\rm LS}}$, where $m$ is the mass of a particle that is considered to be equal for both type of particles, i.e. $m = m_{\rm L} = m_{\rm S} = 1.0$. More details about the model can be found in Ref.[5].

The equation of motions for any particle $i$ located at $\mathbf{r}_i$ and with its neighbour $j$ at $\mathbf{r}_j$:

$$\dot{\mathbf{r}_i} = \frac{\dot{\mathbf{p}}_i}{m_i} \tag{13}$$

and

$$\dot{\mathbf{p}}_i = \sum_{j\neq i}^{N} \mathbf{f}_{(i,j)}^{int} + \mathbf{f}_{(i,j)}^{D} + \mathbf{f}_{(i,j)}^{R} \tag{14}$$

Here, the total force enacted on the particle is a sum over the interaction force, $\mathbf{f}_{(i,j)}^{int} = -\vec{\nabla} V_{\alpha\beta}(\mathbf{r}_{(i,j)})$, the dissipative force, $\mathbf{f}_{(i,j)}^{D} = -\zeta w^2(r_{(i,j)})\,(\hat{\mathbf{r}}_{(i,j)}\,.\,\mathbf{v}_{(i,j)})\hat{\mathbf{r}}_{(i,j)}$ and the random force, $\mathbf{f}_{(i,j)}^{R} = \sqrt{2k_B T}\zeta w(r_{(i,j)})\theta_{(i,j)}\ \hat{\mathbf{r}_{(i,j)}}$. The equations (13-14) ensure the correct thermostatting of the system by canceling the drifting velocities introduced due to shear and warrant Galilean-invariance and conservation of local momenta.

### *Preparation of initial states*

The binary LJ mixture described above is first brought to thermal equilibrium in the supercooled liquid state at $T = 1.08T_{mct}$; where $T_{mct} = 0.325$ is the mode coupling transition temperature for this model. Then corresponding inherent structure (IS) states are generated via a quench to the underlying energy landscape by energy minimization using the conjugate gradient method [2]; these correspond to energy level $E_1 = -2.3254$ (labelled as ESL in the Ref.[2]).

Subsequently, to obtain IS states that are more low-lying in the energy landscape, the supercooled liquid states are cooled into the glassy regime using two different cooling rates, viz. $3.21 \times 10^{-4}, 3.21 \times 10^{-6}$, and the corresponding IS states with respective energy levels $E_2 = -2.3439, E_3 = -2.3771$ are produced via the energy minimization. These states reside in the gap between the states labelled ESL and GQ in Ref.[2].

Thus, we have sampled IS states having very different thermal histories and studied their shear-response.

### *Calculation of shear modulus*

We compute shear modulus from the mechanical response of the sample under quasi-static infinitesimal deformation in athermal conditions for which

$$\mu \approx \lim_{\delta\gamma\to 0} \frac{\delta\sigma_{xy}^{AQS}}{\delta\gamma} \tag{15}$$

where $\delta\sigma_{xy}^{AQS}$ is the shear stress in response to the infinitesimal deformation, $\delta\gamma$ under athermal quasi-static conditions. The measured shear modulus for the states $E_1, E_2, E_3$ are respectively 13.88, 15.29, 18.94.

### *Computing maps of local stress and local yield threshold*

We divide the sample into $M \times M$ square blocks of length $\ell = \frac{L}{M}$, using $M = 32$. We obtain the distribution of the thresholds following "frozen matrix" method[1, 6, 7] by simple shear deformation in the individual blocks. During this process, the neighborhood of the target region remains frozen and deforms affinely while the target region is allowed to relax non-affinely with the onset of plastic rearrangement beyond a local stress threshold, $\sigma_c^{(i,j)}$ via a drop in local stress.

The local shear stress, $\sigma_{xy}^{(n)}$ in a block, $n$ has been computed in the following manner:

$$\sigma_{xy}^{(n)} = \frac{2}{\ell^2}\sum_{i\in n}\sum_{j=1}^{M} \frac{\partial V_{\alpha\beta}(r^{ij})}{\partial r^{ij}} \frac{r_x^{ij} r_y^{ij}}{r^{ij}} \tag{16}$$

following Ref.[1]. The computation of local stresses have been done in the initial state and steady states. Example maps of the local stress and local yield threshold in the initial state are shown in Fig.3, for the different preparation histories studied.

### *Coarse-graining scale*

For coarse-graining the microscopic data from MD simulations to compute the maps discussed above, several coarse graining scales were tested before fixing the scale that we have used, viz. $M \times M = 32 \times 32$. As an example, we show in Fig.4(top), the stress vs strain curves obtained from initial maps using different coarse graining sizes, viz. $M = 16, 32, 64$ which respectively correspond to coarse-graining scales of $\ell = 19.7609, 9.8804, 4.9402$ (in units of $\sigma_{\rm LS}$), for the same initial state (having energy $E_1$). It is evident that the mesh size $32\times 32$ provides the best match of the mesoscale simulations with the MD simulations low shear rate limit. In this limit the value of the overshoot should be solely dependent on the inital condition and thus on the coarse graining size and not on the details in the dynamics.

It is known that the choice of $\ell$ also affects the initial yield stress of a mesoscopic block; a small coarse graining size may overestimate the local threshold due

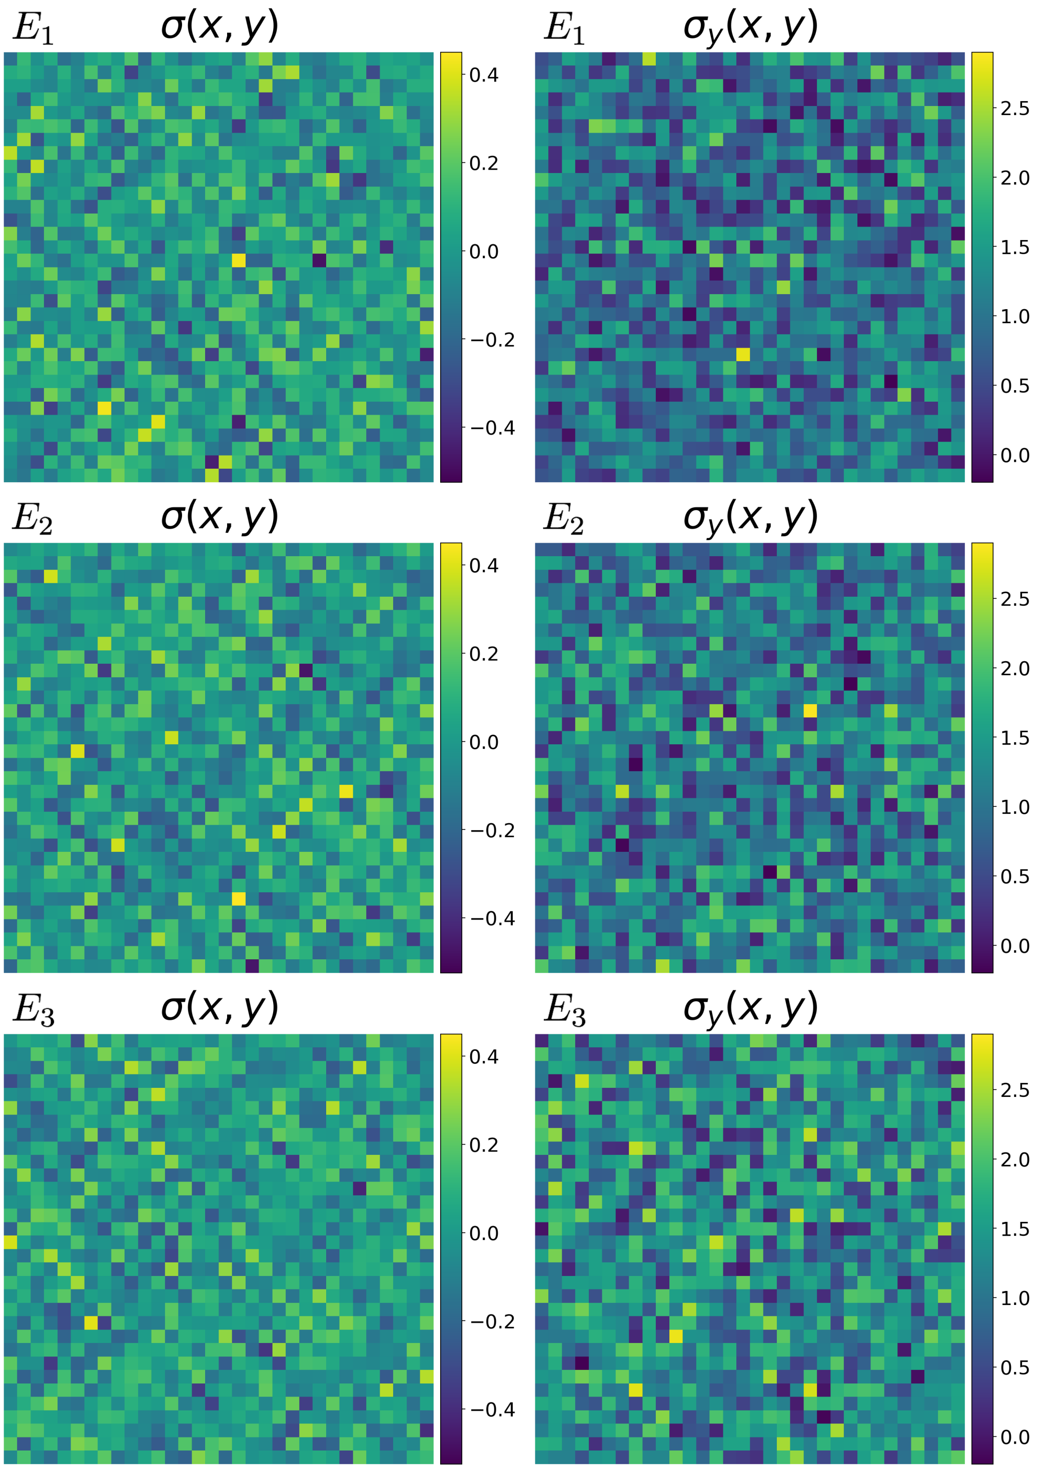


FIG. 3. Maps of (left) coarse-grained stress (right) local yield threshold, constructed from an inherent structure of the microscopic model (discussed in the text) for samples of different thermal histories discussed in this work, viz. $E1, E2, E3$ as labelled, which are used as inputs for the mesoscale calculations. The spatial average of each stress map is zero.

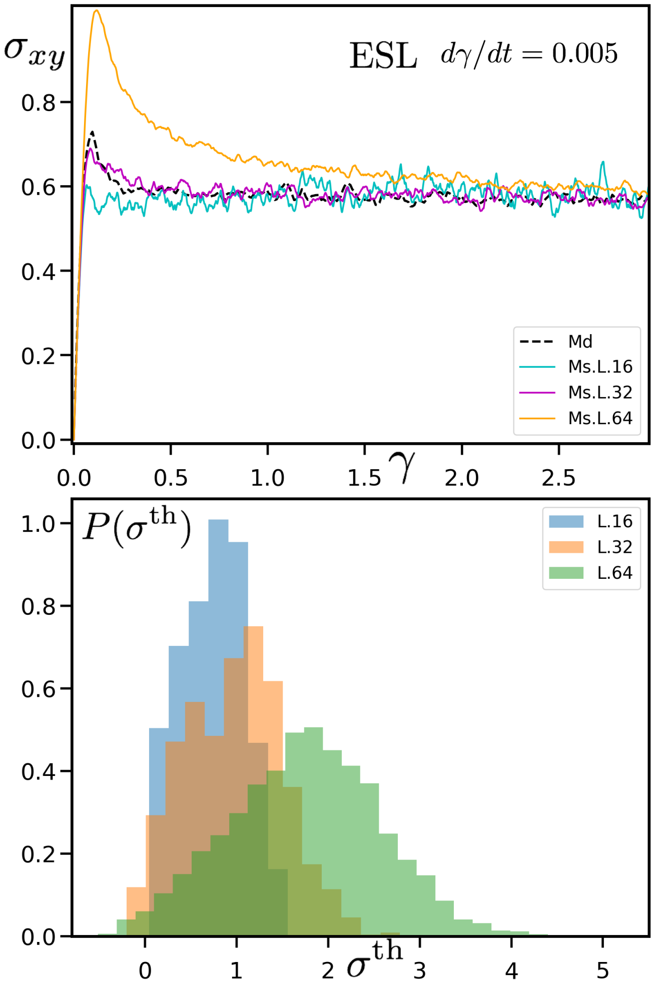


FIG. 4. (Upper panel) For imposed shear rate of $d\gamma/dt = 0.005$, comparison of MD data with load curves obtained from meso scale simulations using different coarse-graining sizes, corresponding deviding the particle based simulation box in $16 \times 16, 32 \times 32, 64 \times 64$ boxes, which respectively correspond to coarse-graining scales of $19.7609, 9.8804, 4.9402$ (in units of $\sigma_{\rm LS}$). The best match is found for the intermediate mesh size corresponding to a division into $32 \times 32$ elementary units. (Bottom panel) Histogram constructed from the initial yield stress field with different coarse-graining sizes. Both plots correspond to system at level $E_1$.

to the frozen matrix [7]. We show our own estimation of the histogram of local thresholds for different coarse graining sizes in Fig.4(bottom). It is clear that smaller the coarse graining scale $\ell$ (i.e. large the mesh size $M$), higher the typical value of local threshold, which is responsible for the mesh size dependence in the load curves in Fig.4(top). Only at reasonable coarse graining size, the typical value of the local threshold gives rise to a macroscopic load curve with a correct overshoot stress. It is also worth noticing that, the coarse graining size found in such way is consistent with the typical size of clusters of particles that undergo Eshelby-like plastic events in amorphous materials, which has been revealed in previous studies [1, 8]. The coarse graining size presented in the our manuscript is thus not only confirmed empirically but also backed up with underlying physical processes.

[1] F. Puosi, J. Olivier, and K. Martens, Probing relevant ingredients in mean-field approaches for the athermal rheology of yield stress materials, Soft matter **11**, 7639 (2015).
[2] S. Patinet, A. Barbot, M. Lerbinger, D. Vandembroucq, and A. Lemaître, On the origin of the bauschinger effect in amorphous solids, arXiv preprint arXiv:1906.09818 (2019).
[3] M. Talamali, V. Petäjä, D. Vandembroucq, and S. Roux, Strain localization and anisotropic correlations in a mesoscopic model of amorphous plasticity, Comptes Rendus Mecanique **340**, 275 (2012).
[4] F. Lançon, L. Billard, and P. Chaudhari, Thermodynamical properties of a two-dimensional quasi-crystal from molecular dynamics calculations, EPL (Europhysics Letters) **2**, 625 (1986).
[5] M. L. Falk and J. S. Langer, Dynamics of viscoplastic deformation in amorphous solids, Physical Review E **57**, 7192 (1998).
[6] P. Sollich, Local strains and yield strains in shear flow of amorphous materials, cecam workshop "multiscale modelling of amorphous materials: from structure to mechanical properties" (ACAM, Dublin, Ireland, 2011).
[7] A. Barbot, M. Lerbinger, A. Hernandez-Garcia, R. García-García, M. L. Falk, D. Vandembroucq, and S. Patinet, Local yield stress statistics in model amorphous solids, Physical Review E **97**, 033001 (2018).
[8] C. A. Schuh, T. C. Hufnagel, and U. Ramamurty, Mechanical behavior of amorphous alloys, Acta Materialia **55**, 4067 (2007).
